# Supplementary material for: HAMSTER: Hierarchical Action Models For Open-World Robot Manipulation
Source: arXiv:2502.05485 source file (2025-05-10)
Supplement: Supplementary file 1 [file appendix_workshop.tex]

\begin{figure}[!t]
    \centering
    \includegraphics[width=\linewidth,trim={0in 1.5in 0in 1.8in},clip]{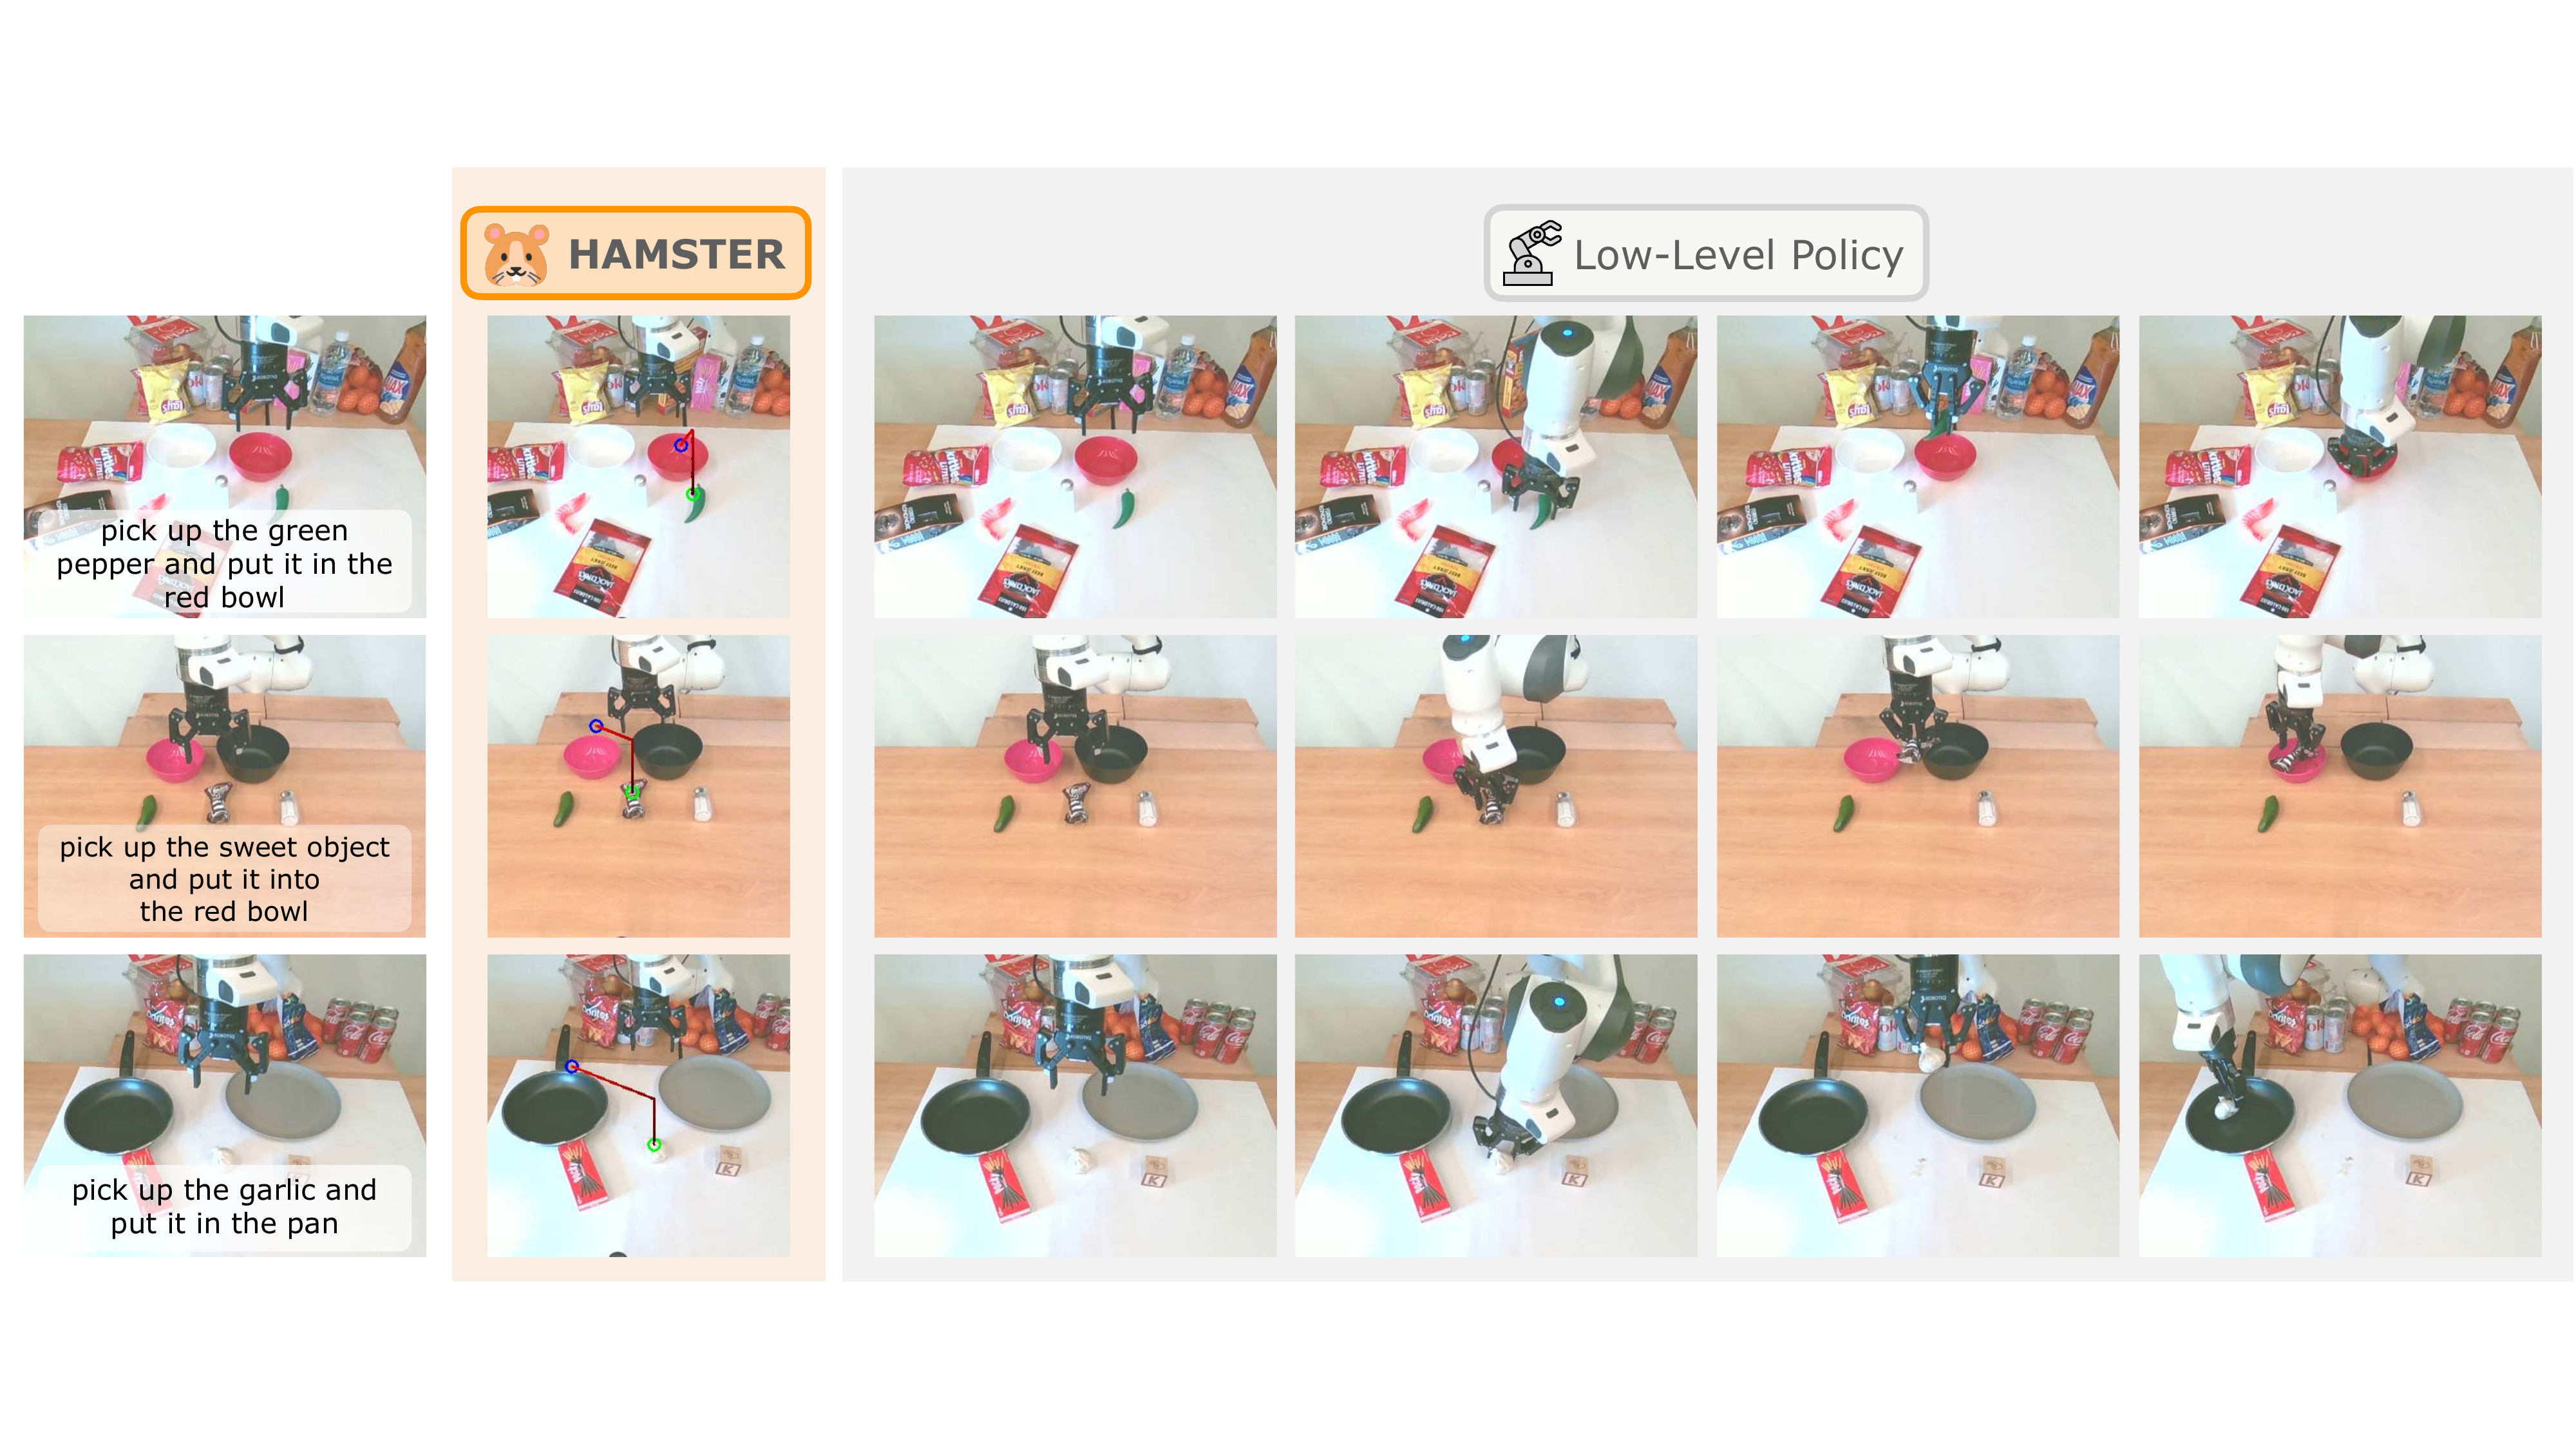}
    \caption{\footnotesize{Example real-world \method\ rollouts demonstrate its strong performance in novel scenes achieved by leveraging VLMs' generalization capabilities and the robust execution of low-level 3D policies.}}
    \label{fig:experiments:real_robot_policy}
    \vspace{-4mm}
\end{figure}

\begin{figure}
    \centering
    \includegraphics[width=\linewidth]{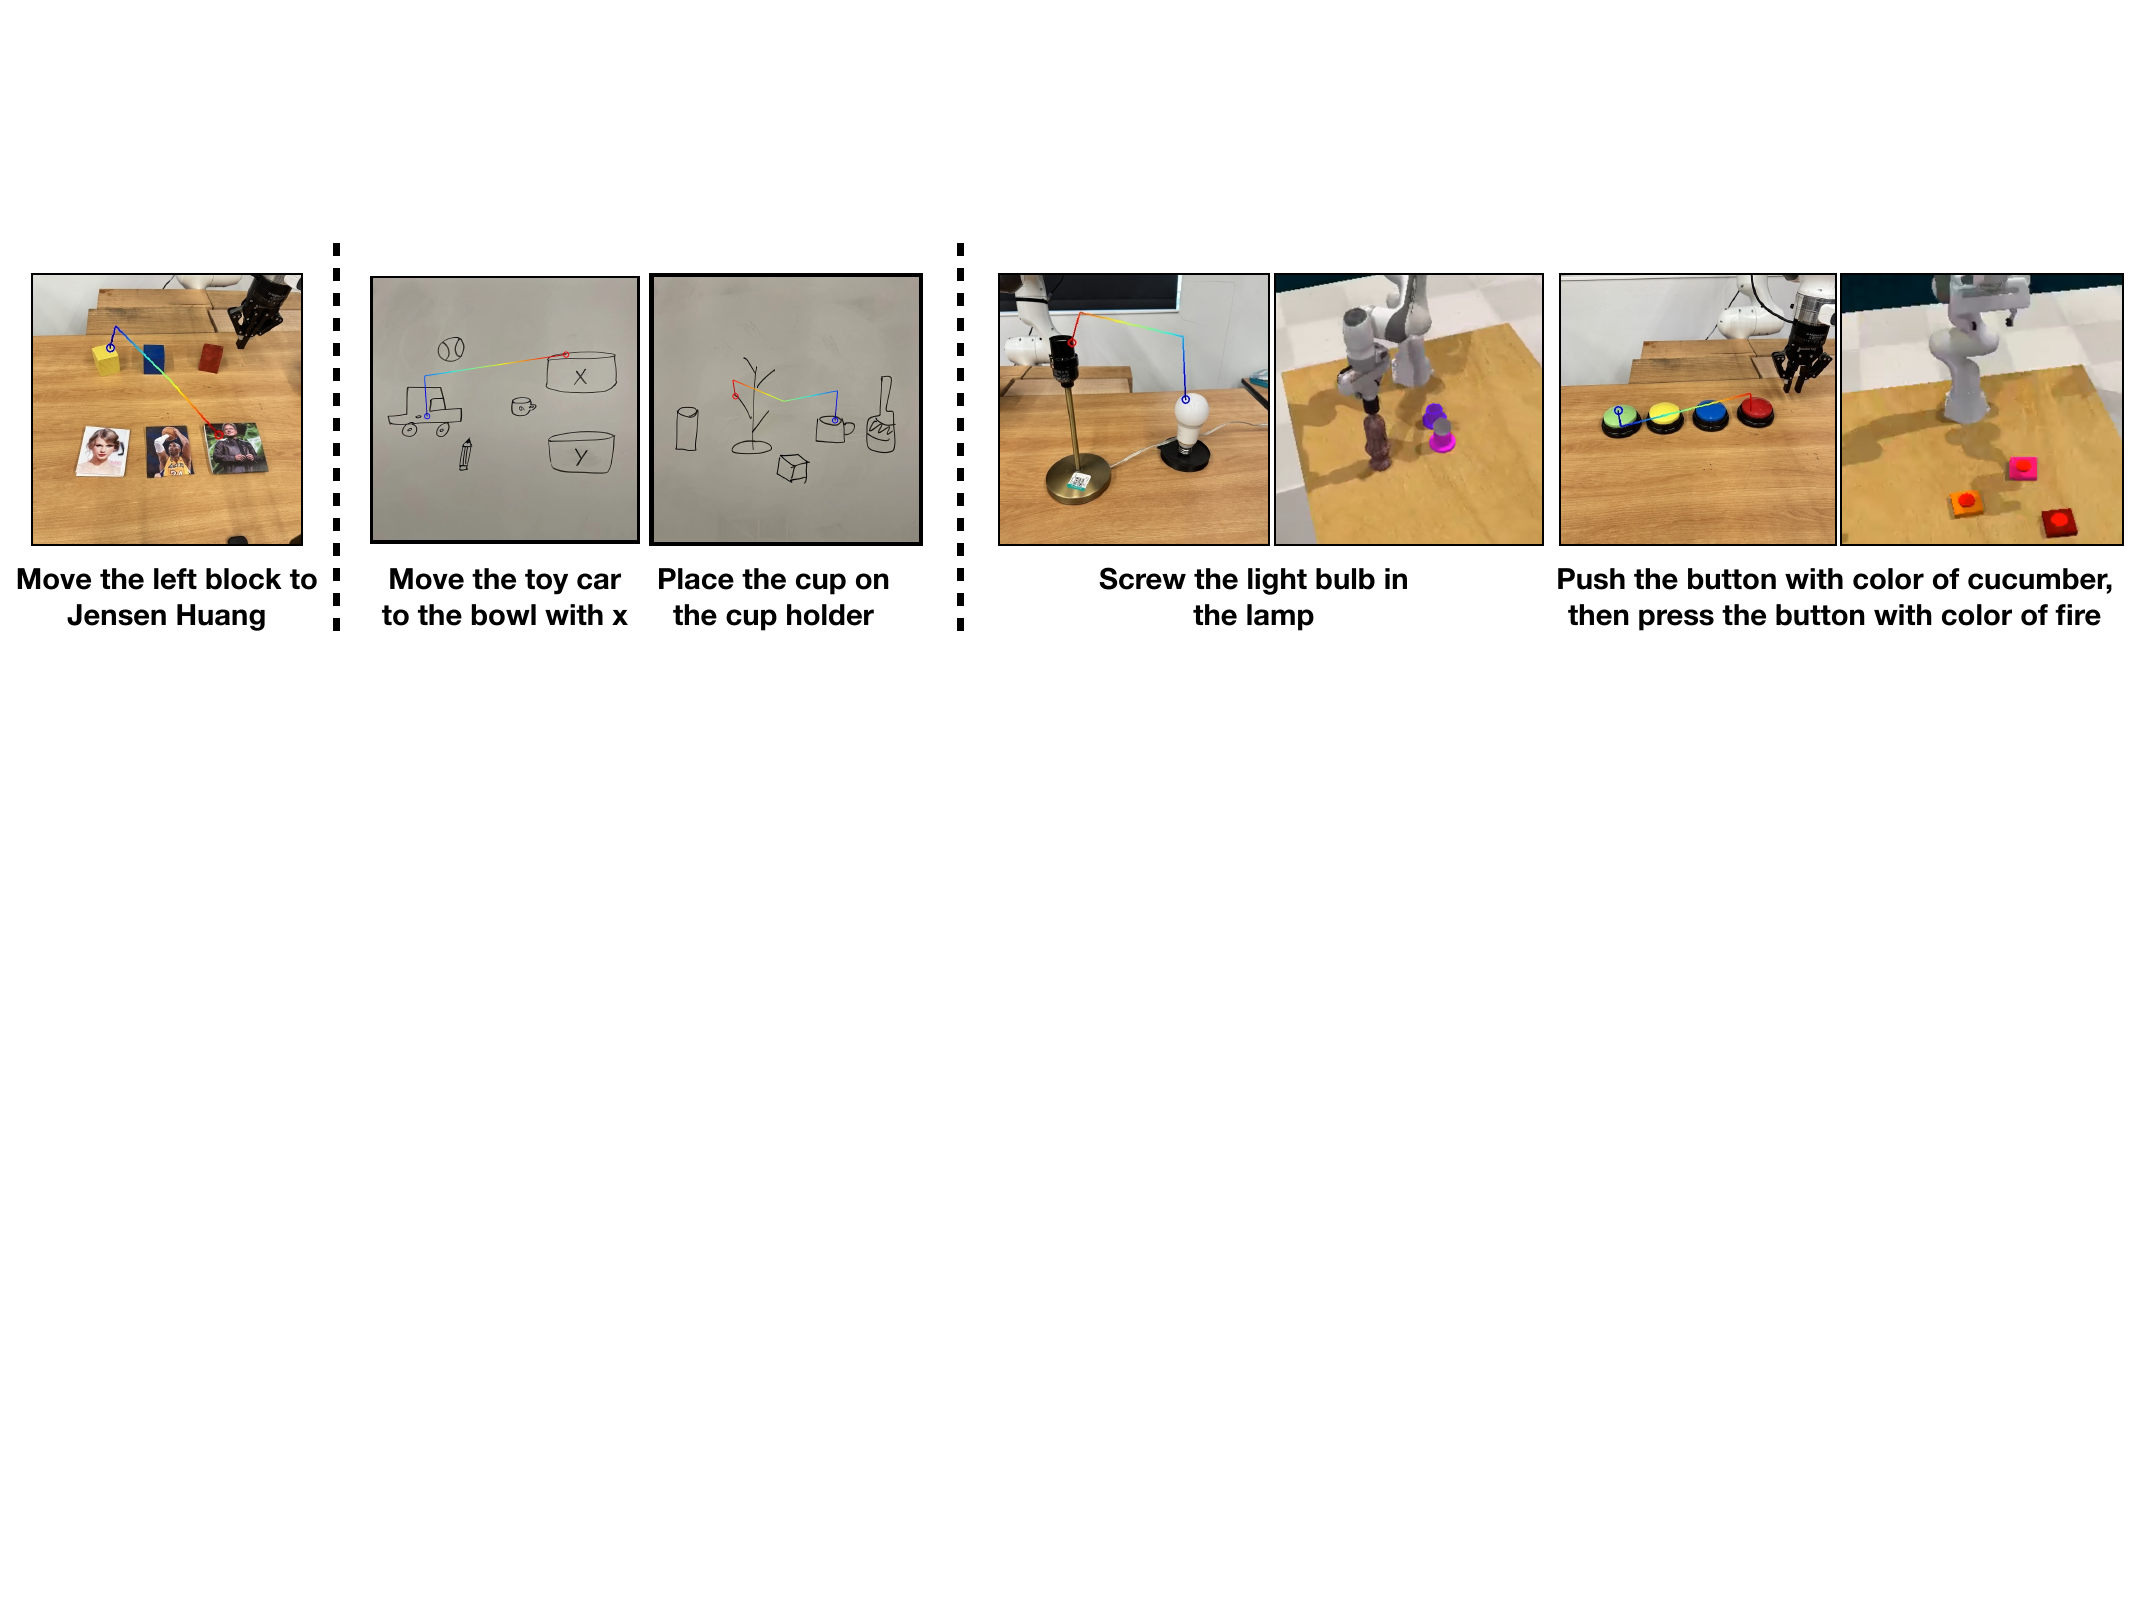}
    \caption{\footnotesize{\method's VLM demonstrates considerable generalization and cross-domain learning to scenarios not encountered in the training set. From left to right: (a) it can effectively utilize world knowledge to generalize to tasks specified by people; (b) it generalizes to highly out-of-domain input images, such as human-drawn sketches; (c) when trained on diverse simulated data it shows transfer to related, but visually distinct tasks in the real world.}}
    \label{fig:vlm_generalization}
    \vspace{-4mm}
\end{figure}

\input{sections/appendix}

\subsection{Simulation Evaluation}
\label{sec:appendix:simulation_results}
We also perform controlled experiments in simulation. We use Colosseum~\citep{pumacay2024colosseum} as the benchmark as it displays considerable visual and semantic variations. In simulation, we paired our high-level VLM, with 3D Diffuser Actor~\citep{ke20243d} as the low-level policy, since this is one of the state-of-the-art models on RLBench. We compare {\method} with a vanilla 3D Diffuser Actor implementation without path guidance. \Cref{tab:experiments:colosseum} summarizes our results in simulation. \method \ significantly outperforms vanilla 3D-DA by 21\%. This shows that the 2D paths produced by the VLM in {\method} can help low-level policies to generalize better to novel unseen variations. We refer readers to \citet{pumacay2024colosseum} for details on the variations and \Cref{sec:appendix:simulation_details} for further details.

\input{tables/colesseum}
